# Supplementary material for: Percolation based architecture for cluster state creation using photon-mediated entanglement between atomic memories
Source: arXiv:1704.07292 ancillary file (2019-08-27)
Supplement: Supplementary file 1 [file supplementary-material.pdf]

**Supplementary Material: Percolation based architecture for  
cluster state quantum computation using photon-mediated  
entanglement between atomic memories**

(Dated: April 24, 2017)

## COLLECTION EFFICIENCY AND ENTANGLEMENT SUCCESS PROBABILITY

The single-photons to be used for entanglement should be spectrally located in the zero phonon line (ZPL). The Debye-Waller factor, the ratio of ZPL emission rate to the total decay rate of the NV center varies from  $3 \sim 5\%$  [S1]. Here, we will use a conservative number:  $3\%$ . In addition to the low fraction of emission in the ZPL, diamonds suffers from low photon collection efficiency because of total internal reflection caused by the high refractive index of diamond. To overcome these issues, various nanophotonic structures for coupling to free space or photonic integrated circuits have been proposed. Here, we consider three collection schemes: free space collection with bullseye grating or solid immersion lens (SIL) [S2], waveguide collection [S3], and high-cooperativity cavity collection [S4].

The Bullseye grating is a circular grating that maximizes free space coupling by interference. Record count rates ( $\sim 2.7 \times 10^6$ ) have been reported with such structures, and simulations have shown  $\sim 30\%$  collection efficiency at the ZPL wavelength. For shallow NV centers within  $\sim 10$  nm from the surface,  $\sim 90\%$  collection efficiency has been estimated. However, we will assume a more conservative number of  $\sim 30\%$  collection efficiency, which results in a ZPL photon collection efficiency of  $1\%$ .

Collection of photons from solid state emitters into waveguides coupled with photonic integrated circuits has been successfully demonstrated [S3, S5]. These collection schemes are more scalable because single photon detectors, filters and beam splitters can be implemented on-chip. In addition, the well-confined optical field makes near unity detection efficiency possible with superconducting nanowire single-photon detectors (SNSPDs) as demonstrated in [S6]. For NV centers, a hybrid approach with silicon nitride (SiN) waveguides successfully showed that the coupling efficiency can be upto  $83\%$ . In this work, a diamond waveguide is *picked and placed* on a SiN waveguide [S3]. Considering the errors in this process, we assumed a conservative photon collection efficiency of  $\sim 66\%$  including detection efficiency.

Lastly, photonic cavities can re-distribute the spectrum of emitted photons, extract them out of the emitter and direct them into the waveguide. When the cavity is tuned to the ZPL wavelength, the Purcell effect enhances emission into the ZPL, resulting in higher conversion efficiency from emitter excitation to ZPL photon. This coherent interaction between the cavity and emitter has been successfully demonstrated in many platforms, and is an area of active research [S4, S5, S7, S8]. We used a number for cooperativity already demonstrated

in ref. [S4]:  $C \sim 1$ . In this paper, a 1-dimensional photonic crystal cavity, which is a natural design for coupling light into a waveguide, was used. By removing a few holes in the Bragg reflector, one can direct photons from the cavity into the waveguide. Including this conversion efficiency, 32% overall collection efficiency is assumed in this paper.

TABLE I. ZPL Collection efficiencies of different schemes

| Collection                          | Bullseye grating (or SIL) | Waveguide | Cavity    |
|-------------------------------------|---------------------------|-----------|-----------|
| ZPL Enhancement                     | $\times$                  | $\times$  | $\sim 33$ |
| Fraction of Emission in the ZPL (%) | 3                         | 3         | 50        |
| Photon Collection Efficiency (%)    | 33                        | 66        | 64        |
| ZPL Collection Efficiency (%)       | 1                         | 2         | 32        |

## PROBABILISTIC BELL MEASUREMENT FOR BROKER QUBIT ENTANGLEMENT

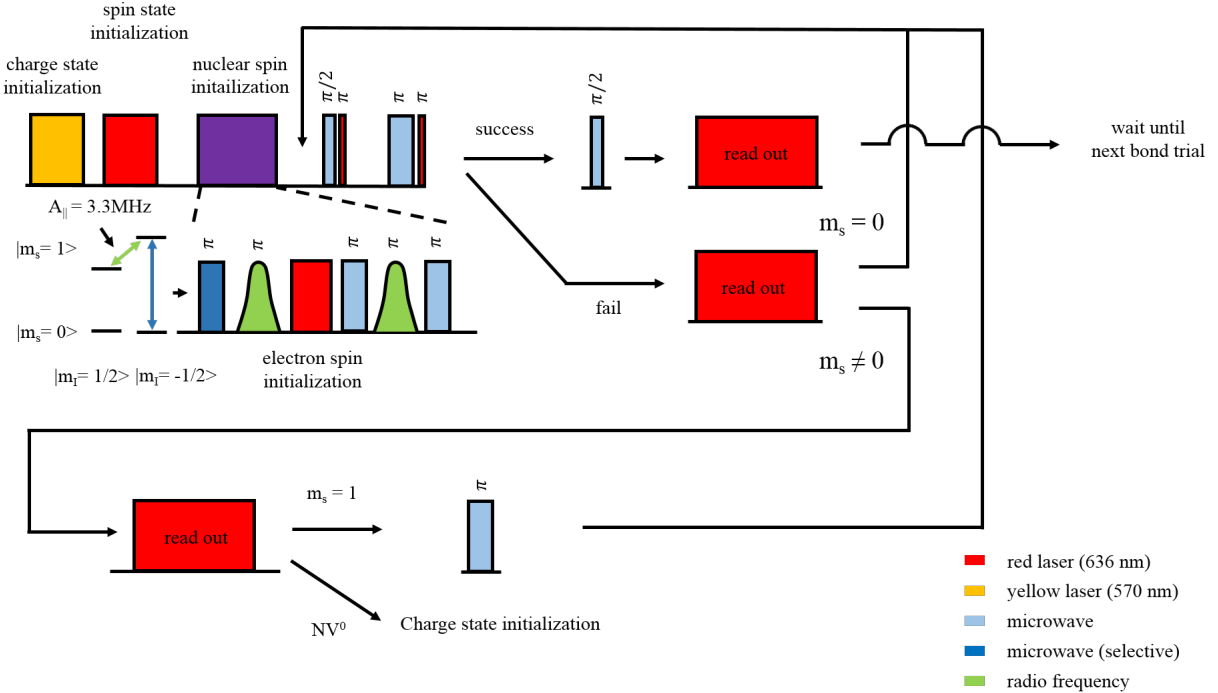

FIG. S1. Pulse sequence for the broker qubit entanglement procedure.

TABLE II. Performance metrics for different collection schemes

| Collection                         | Bullseye           | Waveguide          | Cavity             |
|------------------------------------|--------------------|--------------------|--------------------|
| Bond success prob. $p_0$           | $5 \times 10^{-5}$ | $2 \times 10^{-4}$ | $5 \times 10^{-2}$ |
| Bond trial time $t_0$ <sup>a</sup> |                    | 5 us               |                    |
| Detector jitter                    |                    | $5 \sim 10 ps$     |                    |
| Spectral diffusion                 | $\times$           | $\times$           | $\checkmark$       |
| Readout time                       | 4 us               | 800 ns             | 400 ns             |
| Demonstration                      | Achieved           | Achievable         | Long-term          |

<sup>a</sup> including state initialization

Broker qubits (electronic spin of NV centers) are entangled through Bell measurement (Barret-Kok protocol [S9]), as used in [S1]. The detailed pulse sequence is described in Fig. S1. First,  $\pi/2$ -pulses are applied to both broker qubits. These pulses should be strong enough to drive both hyperfine levels by power broadening, and are represented in light blue, in contrast to the selective pulses denoted in dark blue. An optical  $\pi$ -pulse then reads the states of both spins. Emitted single-photons from the the two electronic spins are then detected after passing through a 50/50 beam-splitter as shown in Fig. 1(d). The beam splitter erases the information of which emitter the detected photon comes from. As a result, a one-photon detection event projects the two spin states into either  $|\psi^+\rangle$  or  $|\psi^-\rangle$  depending on which which detector fired. However, photon loss can cause a two-photon generation event, where the state of the emitters is projected onto  $|00\rangle$ , to be mis-interpreted as a one-photon detection event. In order to overcome this issue, we apply microwave  $\pi$  pulses to each broker qubits. If the emitter was originally projected onto  $|00\rangle$ , this operation changes the emitter state into  $|11\rangle$ . Emission from the two electronic spins is again detected after passing a 50/50 beam splitter. In the case of the desired  $|\psi^+\rangle$  or  $|\psi^-\rangle$  state and no photon loss, a one-photon detection event is registered. The unwanted  $|11\rangle$  state or photon loss leads to no photon detection which we treat as a failed entanglement attempt. Overall, one-photon detection events in both steps makes sure that the two broker qubits are in either  $|\psi^+\rangle$  or  $|\psi^-\rangle$ .

The success probability of the the broker qubit entangling operation  $p$  is determined by the photon collection efficiency  $\eta$ :  $p = \frac{1}{2}\eta^2$  [S9]. The entanglement probability per attempt

is low, but success results in high-fidelity entangled states. This trade-off between success probability and fidelity makes this protocol appealing for our percolation based architecture.

Indistinguishability of photons serves a critical role in Bell measurement. Thus, the wavepackets of the two photons should be perfectly overlapped in the time domain, which can be relatively easily achieved. However, two photons from different emitters should also be overlapped in the frequency domain. In the next paragraphs, we will investigate methods for overcoming two types of frequency mismatch [S10]: static mismatch and dynamic mismatch.

Static mismatch results from the inhomogeneous distribution of the ZPL of NVs, typically caused by local strain. This results in two nearby NVs being detuned upto  $\sim 5$  GHz [S1]. A common misconception is that two photons emitted from different emitters should have the exactly same frequency for indistinguishability. However, this depends on the timing resolution of the photodetectors [S10]. After detection, photons are projected onto a narrow temporal wavepacket that depends on the jitter of the detector. This broadens the distribution in the frequency domain increasing indistinguishability. In other words, the phase difference originating from the difference in photon energy is heralded by the detection time [S10], and can be corrected. In this work, a timing resolution of  $5 \sim 10$  picoseconds is assumed, which has been demonstrated with superconducting nanowire single photon detectors (SNSPD) [S11]. This detector can be both free-space coupled and waveguide-integrated. This detector resolution can easily handle  $\sim 5$  GHz static mismatching. Alternatively, DC stark shift can be used to match the ZPL frequency of two NVs [S1, S12, S13].

Dynamic mismatch is the frequency mismatch originates from fluctuations in the time between different measurements. In contrast to static mismatch, one cannot unwind the phase difference due to dynamic mismatch with good timing resolution detectors, because the frequency difference is unknown. In the case of emitters, this spectral diffusion usually arises from the charge environment of etched surfaces of the nanostructures. As shown in TABLE II, we have assumed that waveguide structures, in which an etched surface is a few hundred nanometers away from the emitter, do not produce spectral diffusion, while in cavity structures, etched surfaces that are only tens of nanometers from an emitter do.

Spectral diffusion can be overcome by the Purcell effect. As analyzed in [S10], the Purcell effect makes the emitter decay faster, so that the effects of spectral diffusion are minimized. A free space lifetime of  $\sim 10$  nsec can tolerate  $\sim 100$  MHz spectral diffusion. If we assume  $C \sim 1$ , the lifetime is reduced by half which can tolerate  $\sim 200$  MHz spectral diffusion.

Chemical surface treatment, such as high temperature annealing [S14], for reducing spectral diffusion is an area of active research. Spectral diffusion of  $\sim 1$  GHz has been observed in NVs near the surface [S15, S16]. We expect a rapid advance in this direction to reduce spectral diffusion under 200 MHz.

Alternatively, we could time-gate the photo-detection by post selection, to fill this gap ( $\sim 200$  MHz vs  $\sim 1$  GHz) e.g. we could only count single-photon detection events that occur within  $\sim 1/5^{th}$  of the lifetime as successes and discard the rest. This will reduce the unknown phase evolution by a factor of 5. Although this will reduce collection efficiency by 80 %, we can still achieve percolation within the coherence time of the nuclear spin.

## ENTANGLEMENT SWAPPING PROCEDURE

When entanglement between electronic spins is successful, the entanglement is transferred to the nuclear spin of NV centers ( $^{15}\text{N}$ ), with a controlled-phase (CZ) gate followed by X basis measurement [S17]. In this way, one can make use of the long coherence time of the nuclear spin with the spin-photon interface of the electronic spin.

Physically, the CZ gate is implemented with a timed-hyperfine interaction with  $A_{||}\tau = \pi$ , where  $\tau$  is the hyperfine interaction time. Since neighboring nodes should be synchronized, the  $^{15}\text{N}$  ( $A_{||} = 3.3$  MHz) nuclear spin is used instead of  $^{13}\text{C}$ , because the  $^{13}\text{C}$  nuclear spin is coupled to the electronic spin with a random strength.  $^{15}\text{NV}$  can be produced by implantation [S18], and its position can be controlled within 10 nm [S19], which is desirable for integration with photonic circuits.

If the probabilistic electronic spin entanglement fails, the next electronic spin entanglement is attempted when  $A_{||}\tau = 2n\pi$ , where  $n$  is an integer, to ensure that the electronic spin is not entangled with the nuclear spin in the case of a failed attempt.

Both electronic spin entanglement and the swapping procedure heralds the exact state of the cluster. Since the heralded state only differs by local Cliffords, they can be compensated in the adaptive measurement steps in the actual computation.

## DETAILS ON THE TIMING OF ENTANGLING OPERATION

The detailed pulse sequence for the whole procedure is described in fig. S1. The charge state is prepared with yellow laser resonant excitation of the  $\text{NV}^0$  ZPL, to minimizing spectral diffusion [S14]. The electronic spin state is then initialized to  $|m_s = 0\rangle$ , by resonantly driving  $|m_s = +1\rangle$  state through the A1 optical transition [S10]. Alternatively, readout with a conditional  $\pi/2$  pulse can be used.  $^{15}\text{N}$  nuclear spin can be initialized to  $|m_I = +1/2\rangle$ , by swapping the nuclear spin with the electronic spin with a nuclear spin conditioned-electronic spin  $\pi$  pulse and electronic spin conditioned-nuclear spin  $\pi$  pulse, and electronic spin initialization.  $|+\rangle_I = (|m_I = +\frac{1}{2}\rangle + |m_I = -\frac{1}{2}\rangle)/\sqrt{2}$  is then prepared by an electronic spin  $\pi$  pulse, nuclear spin  $\pi/2$  pulse and electronic spin  $\pi$  pulse. This whole initialization process is tried only once at the very beginning of the cluster state generation. We assume that all the resonance frequencies are pre-characterized, so that there are negligible errors in the driving.

As specified in the preceding sections, electronic spin entanglement is attempted by two Bell measurements. When the electronic spin entanglement fails, the subsequent electronic spin entanglement attempt should be delayed by  $\tau = 2n\pi/A_{||}$ , where  $n$  is integer number to prevent entanglement of the nuclear and electronic spin. When electronic spin entanglement is successful, the electronic entanglement is swapped to the nuclear spin, the electronic spin is initialized with a conditional  $\pi$  pulse to prevent further hyperfine interaction.

Most of the time, the Bell measurement fails because of low collection efficiency. In this case, electronic spin states are measured and initialized by a conditional optical  $\pi$  pulse. It cannot be directly initialized, as with the very first initialization, because the hyperfine interaction is always on, when electronic spin is non-zero. Therefore, only when the nuclear spin is disentangled with the electronic spin, i.e  $\tau' = 2m\pi/A_{||}$ , where  $m$  is integer, spins are flipped by a timed- $\pi$ -pulse.

In this work, we assumed that two-photon absorption is small enough so that we can ignore charge state conversion, or can account for it with error correction. However, this can be also overcome by (1) reducing resonant laser power and using a weaker pulse, or (2) a timed pulse sequence that can initialize the charge state, while decoupling  $\text{NV}^0$  electronic spin with nuclear spins. This can be done by resonant yellow laser driving and 1064 nm pumping [S20, S21] when  $\tau'' = 2l\pi/A'_{||}$ , where  $A'_{||} = 35.7$  MHz,  $l$  is an integer. This

procedure needs repetition because unlike the resonant excitation, pumping electrons from valence bands is probabilistic.

- 
- [S1] H. Bernien, B. Hensen, W. Pfaff, G. Koolstra, M. S. Blok, L. Robledo, T. H. Taminiau, M. Markham, D. J. Twitchen, L. Childress, and R. Hanson, *Nature* **497**, 86 (2013), arXiv:1212.6136.
  - [S2] L. Li, E. H. Chen, J. Zheng, S. L. Mouradian, F. Dolde, T. Schröder, S. Karaveli, M. L. Markham, D. J. Twitchen, and D. Englund, *Nano Letters* **15**, 1493 (2015).
  - [S3] S. L. Mouradian, T. Schröder, C. B. Poitras, L. Li, J. Goldstein, E. H. Chen, M. Walsh, J. Cardenas, M. L. Markham, D. J. Twitchen, M. Lipson, and D. Englund, *Physical Review X* **5**, 031009 (2015).
  - [S4] L. Li, T. Schröder, E. H. Chen, M. Walsh, I. Bayn, J. Goldstein, O. Gaathon, M. E. Trusheim, M. Lu, J. Mower, M. Cotlet, M. L. Markham, D. J. Twitchen, and D. Englund, *Nature Comm.* **6**, 6173 (2015), arXiv:1409.1602.
  - [S5] A. Sipahigil, R. E. Evans, D. D. Sukachev, M. J. Burek, J. Borregaard, M. K. Bhaskar, C. T. Nguyen, J. L. Pacheco, H. A. Atikian, C. Meuwly, R. M. Camacho, F. Jelezko, E. Bielejec, H. Park, M. Lončar, and M. D. Lukin, *Science* **354** (2016).
  - [S6] F. Marsili, V. B. Verma, J. A. Stern, S. Harrington, A. E. Lita, T. Gerrits, I. Vayshenker, B. Baek, M. D. Shaw, R. P. Mirin, and S. W. Nam, *Nature Photonics* **7**, 210 (2013), arXiv:1209.5774.
  - [S7] A. Faraon, P. E. Barclay, C. Santori, K.-M. C. Fu, and R. G. Beausoleil, *Nature Photonics* **5**, 5 (2010), arXiv:1012.3815.
  - [S8] K. Srinivasan and O. Painter, *Nature* **450**, 862 (2007).
  - [S9] S. D. Barrett and P. Kok, *Physical Review A* **71**, 060310 (2005).
  - [S10] J. Metz and S. D. Barrett, *Physical Review A - Atomic, Molecular, and Optical Physics* **77** (2008), 10.1103/PhysRevA.77.042323.
  - [S11] N. Calandri, Q. Y. Zhao, D. Zhu, A. Dane, and K. K. Berggren, *Applied Physics Letters* **109** (2016), 10.1063/1.4963158, arXiv:1607.06713.
  - [S12] P. Tamarat, T. Gaebel, J. R. Rabeau, M. Khan, A. D. Greentree, H. Wilson, L. C. L. Hollenberg, S. Prawer, P. Hemmer, F. Jelezko, and J. Wrachtrup, *Physical Review Letters*

- 97** (2006), 10.1103/PhysRevLett.97.083002, arXiv:0607170 [quant-ph].
- [S13] V. M. Acosta, C. Santori, A. Faraon, Z. Huang, K.-M. C. Fu, A. Stacey, D. A. Simpson, K. Ganesan, S. Tomljenovic-Hanic, A. D. Greentree, S. Prawer, and R. G. Beausoleil, *Physical Review Letters* **108**, 206401 (2012).
  - [S14] Y. Chu, N. de Leon, B. Shields, B. Hausmann, R. Evans, E. Togan, M. J. Burek, M. Markham, A. Stacey, A. Zibrov, A. Yacoby, D. Twitchen, M. Loncar, H. Park, P. Maletinsky, and M. Lukin, *Nano Letters* **14**, 1982 (2014).
  - [S15] D. Riedel, I. Söllner, B. J. Shields, S. Starosielec, P. Appel, E. Neu, P. Maletinsky, and R. J. Warburton, (2017), arXiv:1703.00815.
  - [S16] T. Ishikawa, K.-M. C. Fu, C. Santori, V. M. Acosta, R. G. Beausoleil, H. Watanabe, S. Shikata, and K. M. Itoh, *Nano Letters* **12**, 2083 (2012).
  - [S17] K. Nemoto, M. Trupke, S. J. Devitt, A. M. Stephens, B. Scharfenberger, K. Buczak, T. Nöbauer, M. S. Everitt, J. Schmiedmayer, and W. J. Munro, *Physical Review X* **4**, 031022 (2014), arXiv:1309.4277.
  - [S18] J. R. Rabeau, P. Reichart, G. Tamanyan, D. N. Jamieson, S. Prawer, F. Jelezko, T. Gaebel, I. Popa, M. Domhan, and J. Wrachtrup, *Applied Physics Letters* **88**, 023113 (2006).
  - [S19] I. Bayn, E. H. Chen, M. E. Trusheim, L. Li, T. Schröder, O. Gaathon, M. Lu, A. Stein, M. Liu, K. Kisslinger, H. Clevenson, and D. Englund, *Nano Letters* **15**, 1751 (2015).
  - [S20] P. Siyushev, H. Pinto, M. Voros, A. Gali, F. Jelezko, and J. Wrachtrup, *Physical Review Letters* **110**, 167402 (2013), arXiv:1204.4898.
  - [S21] P. Ji and M. V. G. Dutt, *Physical Review B* **94**, 024101 (2016).
